# Supplementary material for: SuperFedNAS: Cost-Efficient Federated Neural Architecture Search for On-Device Inference
Source: arXiv:2301.10879 source file (2024-07-11)
Supplement: Supplementary file 1 [file 07-appendix.tex]

\section{Code Release}
We release the code of \proposedfed --- \url{https://anonymous.4open.science/r/FedNASOdin/} . The code includes detailed instructions to run \proposedfed and reproduce the experiments conducted in the paper. 

\section{Supernet FL-Training Algorithms}
\label{app:supernet_training}
We describe in detail the three supernet training algorithms. 

\subsection{Multi-Stage Supernet FL-Training}
\label{app:supernet_training:multi_stage}
\begin{algorithm}[htb]
\footnotesize
   \caption{\small Multi-Stage Supernet FL-Training}
   \label{alg:ps_fl}
\begin{algorithmic}[1]\footnotesize

 \STATE Initialize $W$ \algorithmiccomment{Supernet Weights}
  \FOR{phase p in \{depth, width\}}
  \FOR{round t = 1,2, ... T$_{p}$}
  
   \STATE $\kappa_t \leftarrow$ random set of $max(C\cdot K, 1)$  clients ($\kappa_t \subseteq \kappa$)\algorithmiccomment{randomly pick C.K clients}
%    % \STATE $h_t =$\{(k,$\mathcal{G}(W_t, \alpha_k)$): $k \in \kappa_t$ \& $\alpha_k \in \mathcal{U}(\mathcal{A})$\}  \algorithmiccomment{randomly assign subnets to clients}
   
   \FOR{client $k \in \kappa_t$}
    % \STATE $w^{t}_k \leftarrow h_t(k)$ \algorithmiccomment{clients only receive subnet weights}
%     % , $w^{t}_{k}  \leftarrow \mathcal{G}(W_t, \alpha^{t}_k)$
    \FOR{(x,y) in minibatch($D_k$)}
    \FOR{$\alpha$ in PS-Sample($\mathcal{A}$,p)} 
    % \STATE loss = crossEntropy(forward(x,$\mathcal{G}(W_t, \alpha)$)) \algorithmiccomment{loss on subnet}
    \STATE crossEntropy(forward(x,$\mathcal{G}(W_t, \alpha)$)) 
    \STATE loss.backward() \algorithmiccomment{ gradients of subnet sampled based on phase}
    \ENDFOR
   % \ENDFOR
   \STATE $W^{t+1}_k \rightarrow$ optimizer.step() \algorithmiccomment{clients train supernet locally using PS \cite{ofa}}
  \ENDFOR
  \STATE $W^{t+1} = \frac{1}{|C.K|}\sum_{k \in \kappa_t} \frac{n_k}{n}.W^{t+1}_{k}$ \algorithmiccomment{FedAvg\cite{fedavg} aggregation of supernet weights}
  \ENDFOR
%  % \STATE $W^{0} \leftarrow$ zeros($W_{t}$) \algorithmiccomment{shared-param avg by overlap cardinality}
%  % \STATE $W_{sum}  \leftarrow \sum_{k\in S_t} n_k*\mathcal{M}(W^{0},\;arch^{k}_t ,\;w^{k}_{t+1})$
%  % \STATE $W_{sum} \leftarrow $  replace\_zeros($W_{sum}$, $W_t$) %
%  % \STATE $W_{cnt} \leftarrow \sum_{k\in S_t} \mathcal{M}(W^{0}, arch^{k}_t , n_k*ones(w^{k}_{t+1}))$
%  % \STATE $W_{cnt} \leftarrow $  replace\_zeros($W_{cnt}$, $1$) %
%  % \STATE $W_{t+1} \leftarrow \frac{W_{sum}}{W_{cnt}}$
\ENDFOR
\ENDFOR
\end{algorithmic}
\end{algorithm}
% \vspace{-0.1in}

Algorithm~\ref{alg:ps_fl} lists multi-stage supernet FL-training.  The training algorithm runs on multiple phases (line 2 in Algorithm\ref{alg:ps_fl}). Within each phase, the clients receive the supernet and perform phased-based sampling in each minibatch to train the supernet locally  (lines 7-9 in Algorithm~\ref{alg:ps_fl}). The phased-based sampling is directly borrowed from OFA \cite{ofa}. Once the supernet gets trained locally by clients, the supernet weights are averaged similar to FedAvg \cite{fedavg}. Note that PS-based sampling (line 7 in Alg~\ref{alg:ps_fl}) adds more computational cost in each local epoch.
\payman{Either use Algorithm or Alg.!}
\subsection{Single Stage Supernet FL-Training}
\label{app:supernet_training:single_stage}
\begin{algorithm}[htb]
\footnotesize
   \caption{\small Single-Stage Supernet FL-Training}
   \label{alg:single_stage}
\begin{algorithmic}[1]\footnotesize

 \STATE Initialize $W$ \algorithmiccomment{Supernet Weights}

  \FOR{round t = 1,2, ... T}
   \STATE $\kappa_t \leftarrow$ random set of $max(C\cdot K, 1)$  clients ($\kappa_t \subseteq \kappa$)\algorithmiccomment{randomly pick C.K clients}
   \STATE $h_t =$\{(k,$\mathcal{G}(W_t, \alpha_k)$): $k \in \kappa_t$ \& $\alpha_k \in \mathcal{U}(\mathcal{A})$\}  \algorithmiccomment{randomly assign subnets to clients}
   
   \FOR{client $k \in \kappa_t$}
    \STATE $w^{t}_k \leftarrow h_t(k)$ \algorithmiccomment{clients only receive subnet weights}
    % , $w^{t}_{k}  \leftarrow \mathcal{G}(W_t, \alpha^{t}_k)$
   \STATE $w^{t+1}_{k} \leftarrow$  ClientUpdate(k ,$w^{t}_{k}$) \algorithmiccomment{train subnet locally}
  \ENDFOR
  \STATE $W^{t+1} = \frac{\sum_{k \in \kappa_t} \frac{n_k}{n}.w^{t+1}_{k}}{\sum_{k \in \kappa_t}|w^{t+1}_{k}|}$ \algorithmiccomment{cardinal averaging of subnet weights onto supernet}
 % \STATE $W^{0} \leftarrow$ zeros($W_{t}$) \algorithmiccomment{shared-param avg by overlap cardinality}
 % \STATE $W_{sum}  \leftarrow \sum_{k\in S_t} n_k*\mathcal{M}(W^{0},\;arch^{k}_t ,\;w^{k}_{t+1})$
 % \STATE $W_{sum} \leftarrow $  replace\_zeros($W_{sum}$, $W_t$) %
 % \STATE $W_{cnt} \leftarrow \sum_{k\in S_t} \mathcal{M}(W^{0}, arch^{k}_t , n_k*ones(w^{k}_{t+1}))$
 % \STATE $W_{cnt} \leftarrow $  replace\_zeros($W_{cnt}$, $1$) %
 % \STATE $W_{t+1} \leftarrow \frac{W_{sum}}{W_{cnt}}$
\ENDFOR
\end{algorithmic}
\end{algorithm}
% \vspace{-0.1in}

Algorithm~\ref{alg:single_stage} lists the training algorithm for training the supernets in a single stage. In this algorithm, the subnets are randomly sampled and given to clients (line 4 in Algorithm~\ref{alg:single_stage}). The clients train the subnets locally (line 7 in Algorithm~\ref{alg:single_stage}). Once the subnets are trained the clients perform cardinal averaging: a parameter that is shared by multiple subnets gets averaged more (line 9 in Algorithm~\ref{alg:single_stage}). Overall, since subnets are distributed to clients in this training algorithm, it has less communication and computational cost.

\subsection{\proposedTraining's FL Supernet Training}
\label{app:supernet_training:maxnet}
\begin{algorithm}[htb]
\footnotesize
   \caption{\small \proposedTraining's Supernet FL-Training}
   \label{alg:maxnet}
\begin{algorithmic}[1]\footnotesize

 \STATE Initialize $W$ \algorithmiccomment{Supernet Weights}
 \STATE CNT$_{\alpha_{max}}$,CNT$_{\alpha_{min}}$ = \{k:0 for $k \in \kappa$\}\algorithmiccomment{tracker for min/max subnet assignment}
 \STATE Initialize $\beta$\algorithmiccomment{Initial value for Maxnet's hyper-param}

  \FOR{round t = 1,2, ... T}
   \STATE $\kappa_t \leftarrow$ random set of $max(C\cdot K, 1)$  clients ($\kappa_t \subseteq \kappa$)\algorithmiccomment{randomly pick C.K clients}
   \STATE k$_{{max}}$ = argmin$_{k \in \kappa_t}$ CNT$_{\alpha_{max}}$[k] \algorithmiccomment{client with least assignment of max subnet}
   \STATE k$_{{min}}$ = argmin$_{k \in \kappa_t}$ CNT$_{\alpha_{min}}$[k] \algorithmiccomment{client with least assignment of min subnet} 
   \STATE $h_t =$ ($k_{{max}}$,$\mathcal{G}(W_t, \alpha_{max})$) $\cup$ ($k_{{min}}$,$\mathcal{G}(W_t, \alpha_{min})$)\algorithmiccomment{assign max,min subnets}
   \STATE $h_t =$\{(k,$\mathcal{G}(W_t, \alpha_k)$): $k \in \kappa_t \setminus \{k_{{min}},k_{{max}}\}$ \& $\alpha_k \in \mathcal{U}(\mathcal{A})$\}  \algorithmiccomment{randomly assign subnets to rest of the clients}
   
   \FOR{client $k \in \kappa_t$}
    \STATE $w^{t}_k \leftarrow h_t(k)$ \algorithmiccomment{clients only receive subnet weights}
    % , $w^{t}_{k}  \leftarrow \mathcal{G}(W_t, \alpha^{t}_k)$
   \STATE $w^{t+1}_{k} \leftarrow$  ClientUpdate(k ,$w^{t}_{k}$) \algorithmiccomment{train subnet locally}
  \ENDFOR
  % \STATE $W^{t+1}=$ $\frac{\beta. \frac{n_{k_{\alpha_{max}}}{} .w^{t+1}_{k_{\alpha_{max}}} + (1-\beta).\sum_{k \in \kappa_t \setminus \{k_{\alpha_{max}}\} }   }  }{}$
  \STATE  $W^{t+1}=$ $\frac{ \beta_t. \frac{n_{k_{{max}}}}{n}. w^{t+1}_{k_{{max}}}   + (1-\beta_t).\sum_{k \in \kappa_t \setminus \{k_{{max}}\} } \frac{n_k}{n}.w^{t+1}_k }{\beta_t. |w^{t+1}_{k_{{max}}}|   + (1-\beta_t).\sum_{k \in \kappa_t \setminus \{k_{{max}}\} } .|w^{t+1}_k| }$ \algorithmiccomment{wt. cardinal averaging}
  \STATE CNT$_{\alpha_{max}}$[k$_{{max}}$] += 1, CNT$_{\alpha_{min}}$[k$_{{min}}$] += 1 \algorithmiccomment{update counters}
  \STATE $\beta_{t+1}$ = decay($\beta_t$, t) \algorithmiccomment{decay $\beta$}
  % \STATE $W^{t+1} = \frac{\beta.\frac{n_{k_{\alpha_{max}}}}{n}.w^{t+1}_{k_{\alpha_{max}}}+ (1-\beta).\sum_{k \in \kappa_t\setminus\{k_{\alpha_{max}}\} w^{t+1}_{k_{\alpha_{max}}}
  % + (1-\beta).k_{\alpha_{max}}\}}w^{t+1}_{k}}{\sum_{k \in \kappa_t\setminus\{k_{\alpha_{max}}\}}|w^{t+1}_{k}|}$ \algorithmiccomment{cardinal averaging of supernet weights}
 % \STATE $W^{0} \leftarrow$ zeros($W_{t}$) \algorithmiccomment{shared-param avg by overlap cardinality}
 % \STATE $W_{sum}  \leftarrow \sum_{k\in S_t} n_k*\mathcal{M}(W^{0},\;arch^{k}_t ,\;w^{k}_{t+1})$
 % \STATE $W_{sum} \leftarrow $  replace\_zeros($W_{sum}$, $W_t$) %
 % \STATE $W_{cnt} \leftarrow \sum_{k\in S_t} \mathcal{M}(W^{0}, arch^{k}_t , n_k*ones(w^{k}_{t+1}))$
 % \STATE $W_{cnt} \leftarrow $  replace\_zeros($W_{cnt}$, $1$) %
 % \STATE $W_{t+1} \leftarrow \frac{W_{sum}}{W_{cnt}}$
\ENDFOR
\end{algorithmic}
\end{algorithm}
% \vspace{-0.1in}

Algorithm~\ref{alg:maxnet} lists the \proposedTraining's training algorithm. \proposedTraining minimizes the loss of worst-performing subnets on each data partition and prioritizes sampling of larger subnets. To approximate this, it keeps track of the minimum and maximum subnets assigned to each client (line 2 in Algorithm~\ref{alg:maxnet}). In each round, it finds the clients that received the minimum and maximum the least (lines 6-7 in Algorithm~\ref{alg:maxnet}). For the rest of the clients, the subnets are randomly assigned (line 9 in Algorithm~\ref{alg:maxnet}). The subnets are trained locally by each client. Once the subnets are trained, \proposedTraining performs weighted cardinal averaging (line 14 in Algorithm~\ref{alg:maxnet}) using $\beta_t$. This is done to emulate the weight-shared-based probability sampling. Finally, the $\beta_t$ is decayed per round based on a decay function, and the trackers for minimum/maximum subnets are updated.

\begin{figure*}[t]
% \vspace{-0.7cm}
    \centering
    \begin{subfigure}[b]{0.45\textwidth}
        \includegraphics[width=\textwidth]{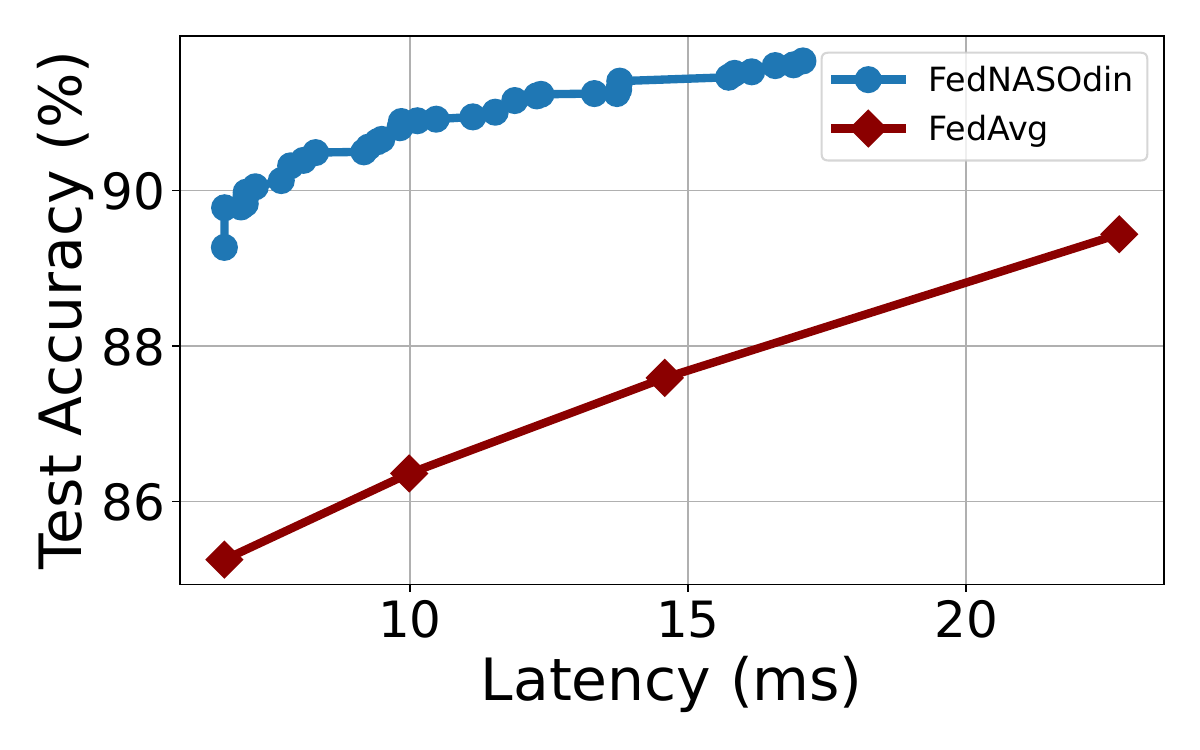} % Adjust the height as needed
        \caption{RTX 2080Ti}
        \label{fig:nas_pareto:cpu}
    \end{subfigure}
    \hfill
    \begin{subfigure}[b]{0.45\textwidth}
        \includegraphics[width=\textwidth]{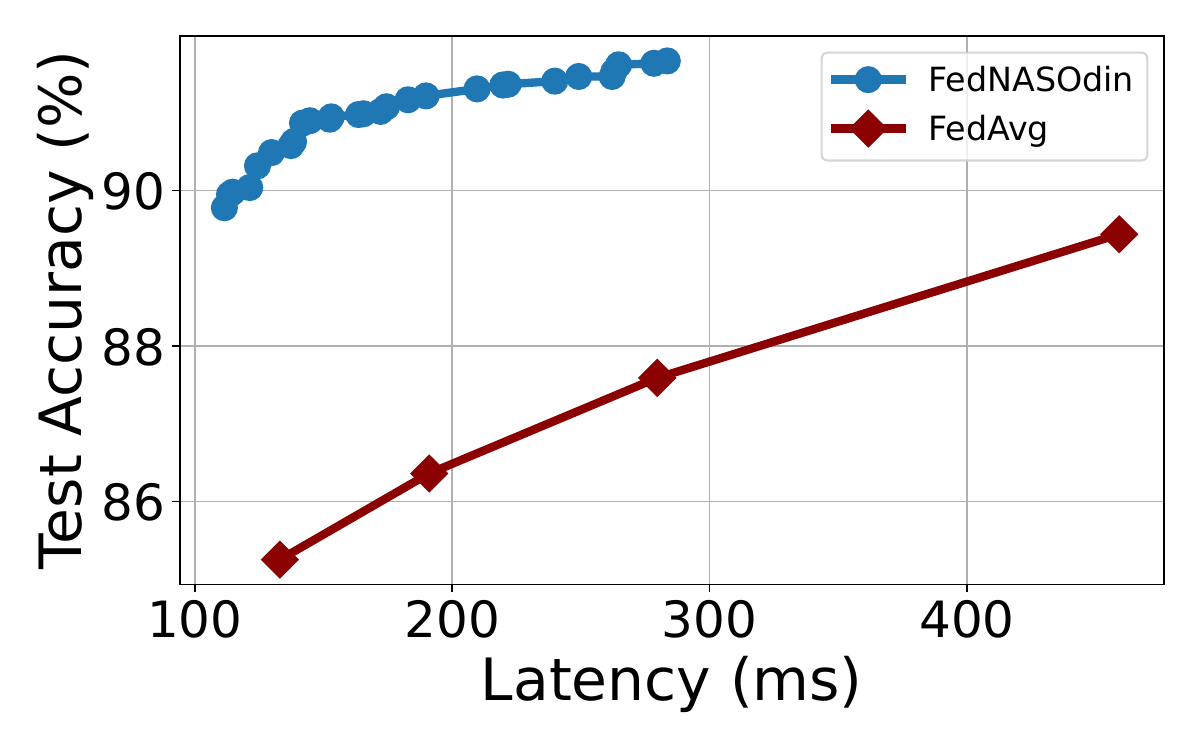}
        \caption{AMD CPU}
        \label{ffig:nas_pareto:gpu}
    \end{subfigure}
    % \hfill
    % \begin{subfigure}[b]{0.37\textwidth}
    %     \includegraphics[width=\textwidth]{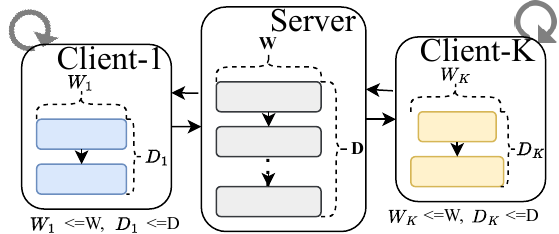}
    %     \caption{Naive Single-Stage Supernet FL}
    %     \label{fig:single_stage}
    % \end{subfigure}
    % \vspace{-2ex}
    \caption{\small \textbf{\proposedfed's Pareto-Optimal Subnets for Target Hardware}  \proposedfed's search stage trains and searches for Pareto optimal subnets for different target hardware compared manually trained DNNs (using scaling rule \cite{efficient_net}) with FedAvg \cite{fedavg}.}  
    % architecture (with 85.25\% accuracy) for 112 ms latency target on AMD CPU and wide/deep DNN architecture (with 91.56\% accuracy) for 18.2 ms latency target on RTX 2080Ti GPU.} 
    \label{fig:nas_pareto}
     % \vspace{-0.7cm}
     % \vspace{-2ex}
\end{figure*}

\section{\proposedfed's NAS results on Different hardware}
\label{app:nas_results}
\figref{fig:nas_pareto} shows Pareto-optimal subnets found by \proposedfed on two different target hardware: AMD CPUs and RTX2080Ti GPU. The figure also compares \proposedfed with training manually designed DNN architectures (using scaling rule \cite{efficient_net}) with FedAvg. The experiment is done on CIFAR10 dataset partitioned into $K=20$ clients and 40\% client participation. 

\noindent \textit{Takeaway.} \proposedfed's finds specialized DNNs for target hardware with better accuracy/latency trade-offs. It achieves up to 4\% more accuracy for the same latency or 3x latency reduction for the same accuracy. This also demonstrates the efficacy of training supernets using \proposedTraining as it reduces interference. The search time of \proposedfed's is minimal as it does not involve any re-training.

\section{Text Dataset Details}
\label{app:text}

In this section, we describe our TCN \cite{tcn} supernetwork and local training hyper-parameters associated with the text dataset experiment. 

\subsection{DNN Architecture Space: Supernet Based on TCNs}
\label{app:text:arch}
The TCN architecture \citep{tcn} for Shakespeare dataset (LEAF) \cite{leaf} consists of eight layers (or four temporal blocks) with 600 input and output channels. We enable two elastic dimensions in the TCN architecture --- depth and expand ratio. Depth defines the the number of blocks to be activated whereas the expand ratio defines the number of output channels of the first layer of each block. Overall, the depth choices considered are \{0,1,2\} with $0$ denoting activating the top two blocks only, and expand ratio choices are \{0.1, 0.2, 0.5, 1.0\}.

\subsection{Local Training Hyper-params} 
\label{app:text:hyper}
For client local training in the text dataset, the initial learning rate is kept at four. We decay the learning rate every 50 local epochs by 0.1. We use gradient norm clipping as $0.05$ and batch size 32. We run five local epochs per client for every communication round.

\section{Training Cost calculation}
\label{appendix:cost_calc}
\subsection{Computational Cost}
We define computational cost as the computations done by the client in FL training. Hence, we estimate computational cost in a supernet FL training. Note that the cost is proportional to the MACs of the model (subnetwork) that it is training. The sum of MACs of all the subnetworks that each client sees throughout the training procedure is reported. 
% Then, an average is calculated over the total number of clients and the total number of communication rounds.
% \\
% \textbf{\fedalg.} Sum of GFLOPs of all the subnetworks that each clients sees over the course of training procedure is done. Then, an average is calculated over the total number of clients and total number of communication rounds.
% \\
% \textbf{\fedinf.} Here all the subnetworks of a model family are trained independently. The GFLOPs of a subnetwork is proportional to the time client spends per round in \fedavg training . Hence, the sum of GFLOPs of all subnetworks in the family is the average computational cost per round in \fedinf. 

\subsection{Communication Cost}
Communication cost is defined by the average bytes transferred between the clients and the server in FL training. The total communication cost is the sum of communication costs per round. Hence, we first calculate the average communication cost per FL round. The average includes both the download and upload of the model. The bytes are transferred to the clients and vice-versa depending on the size of the subnetwork. The sum of the size (in GB) of subnetworks distributed to each client at each communication round is calculated. 

\section{Client Class Distribution}
\label{app:client_class_dist}
\begin{figure*}[h!]
	\centering
	\begin{subfigure}[b]{0.3\textwidth}

        \includegraphics[width=1\textwidth]{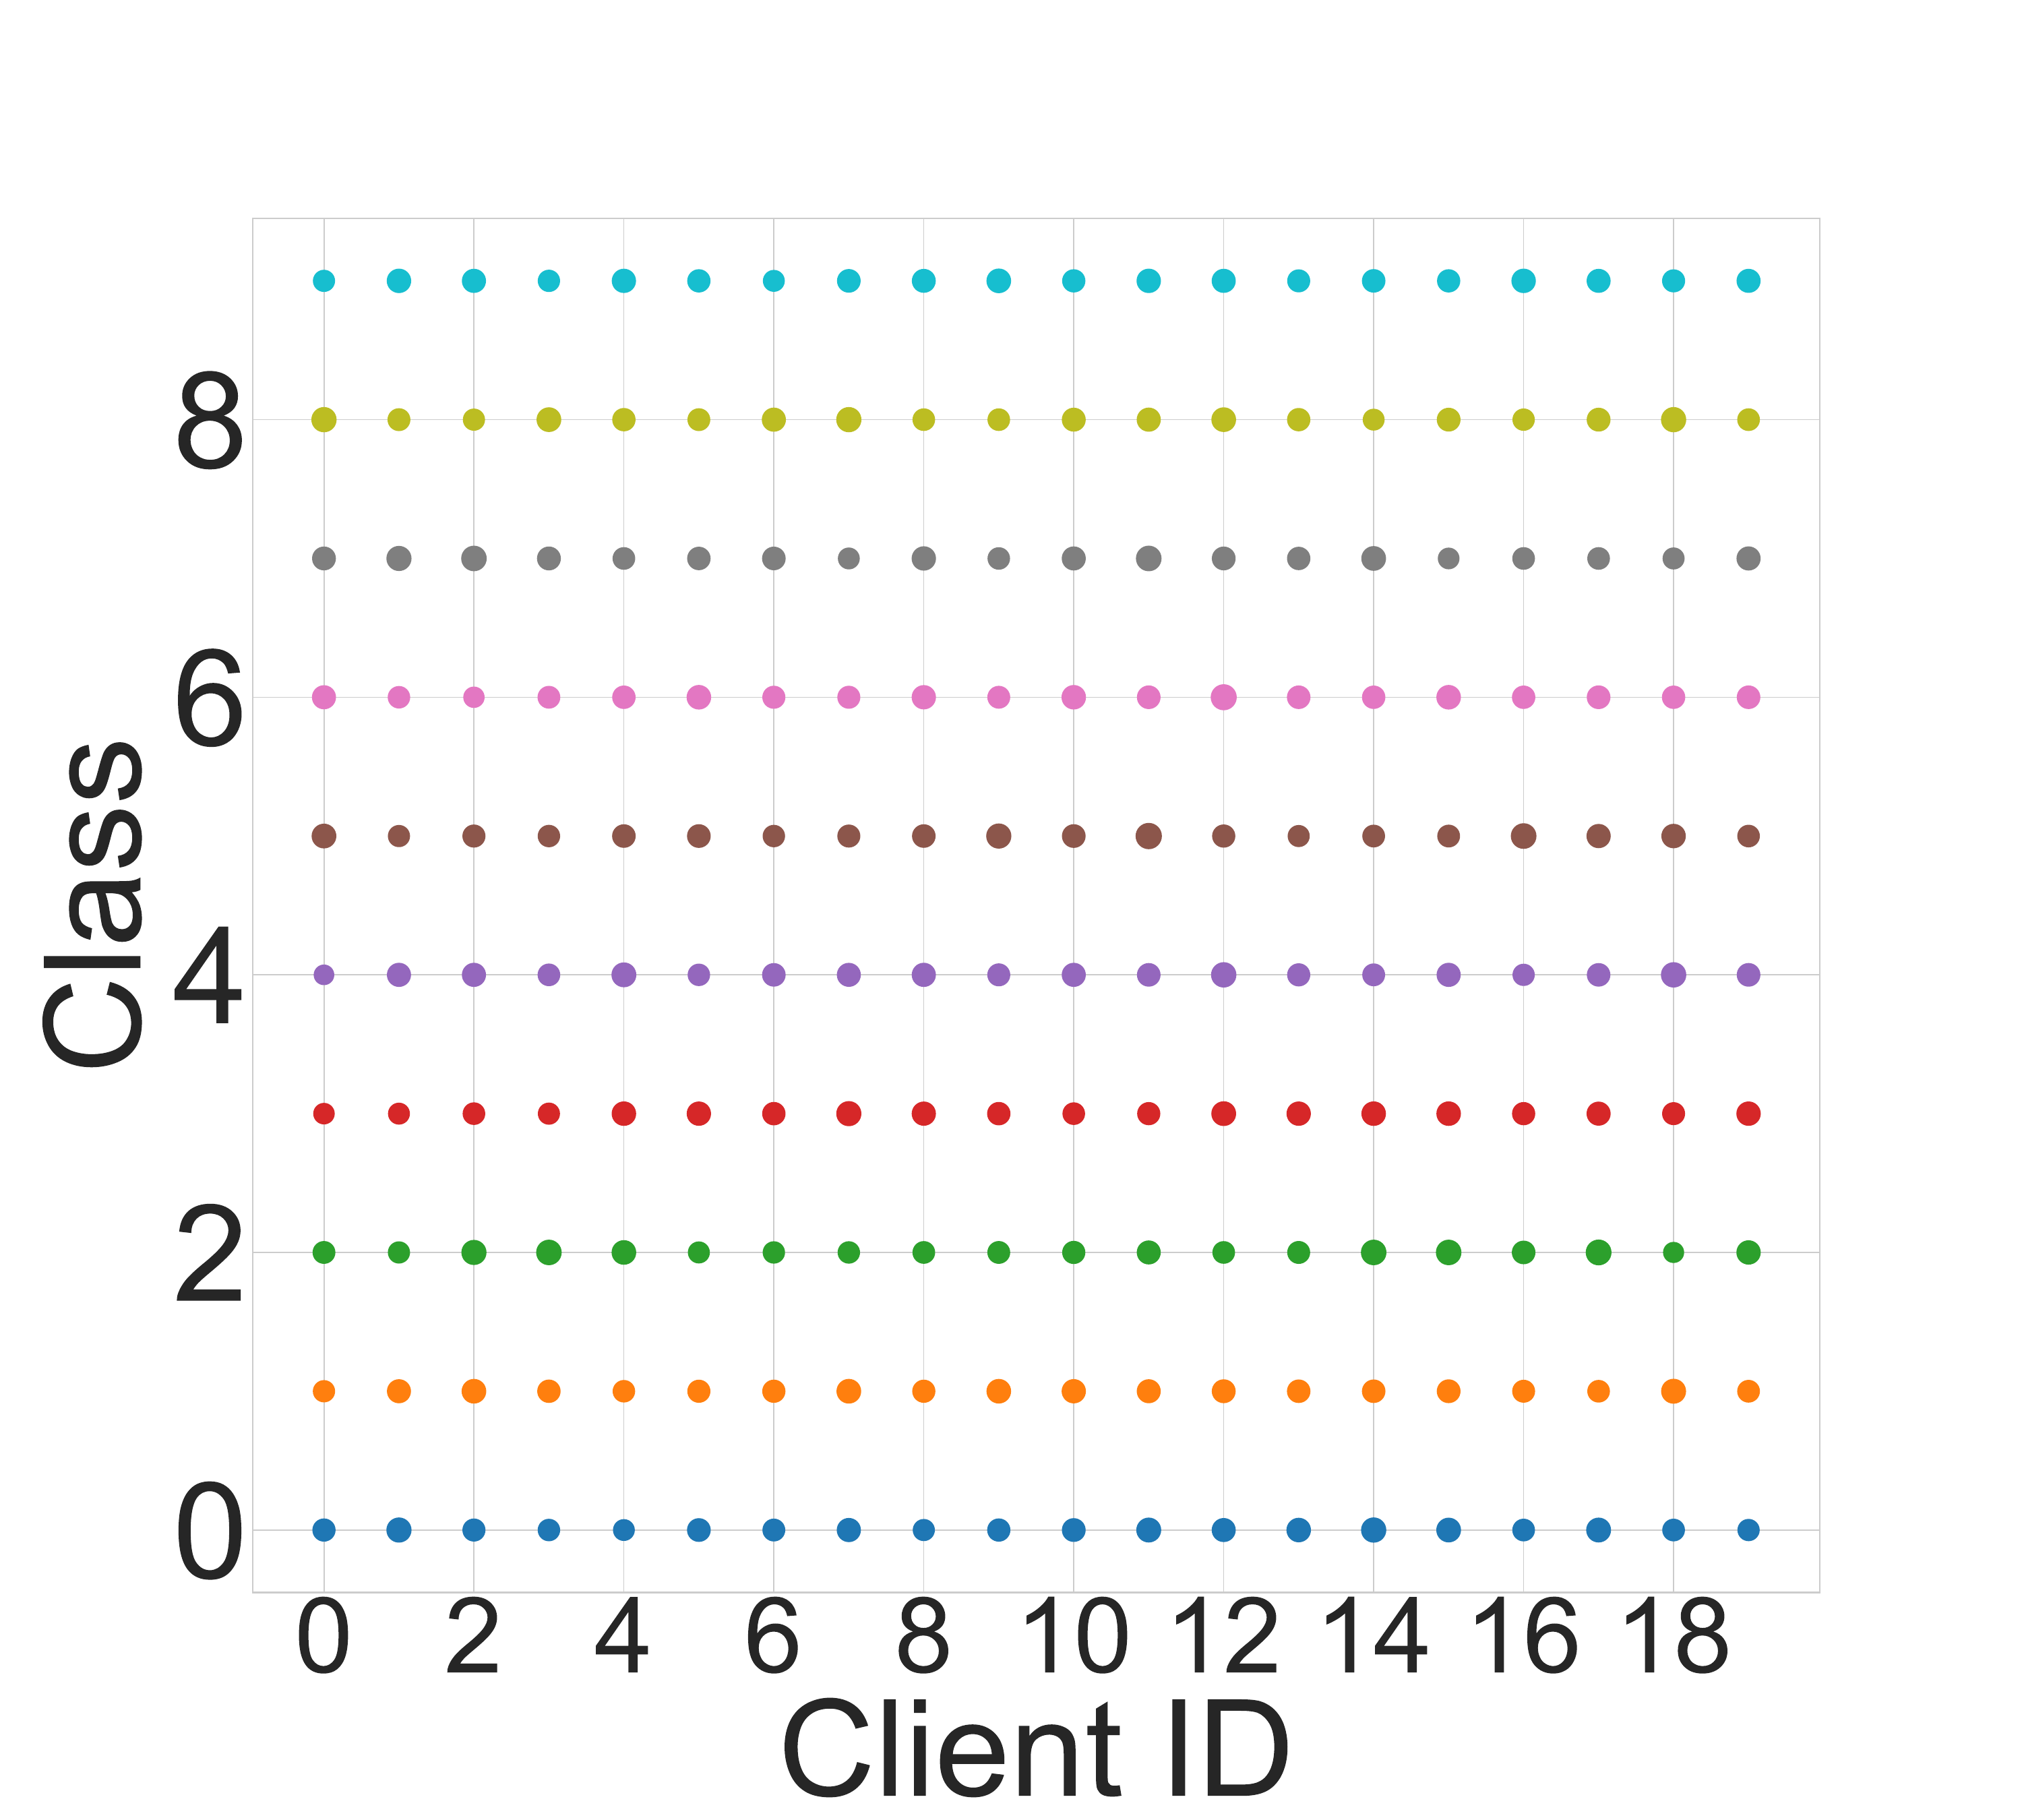}
	    \caption{
		     non-iid=100.
		}
	\end{subfigure}
	\begin{subfigure}[b]{0.3\textwidth}
        \includegraphics[width=1\textwidth]{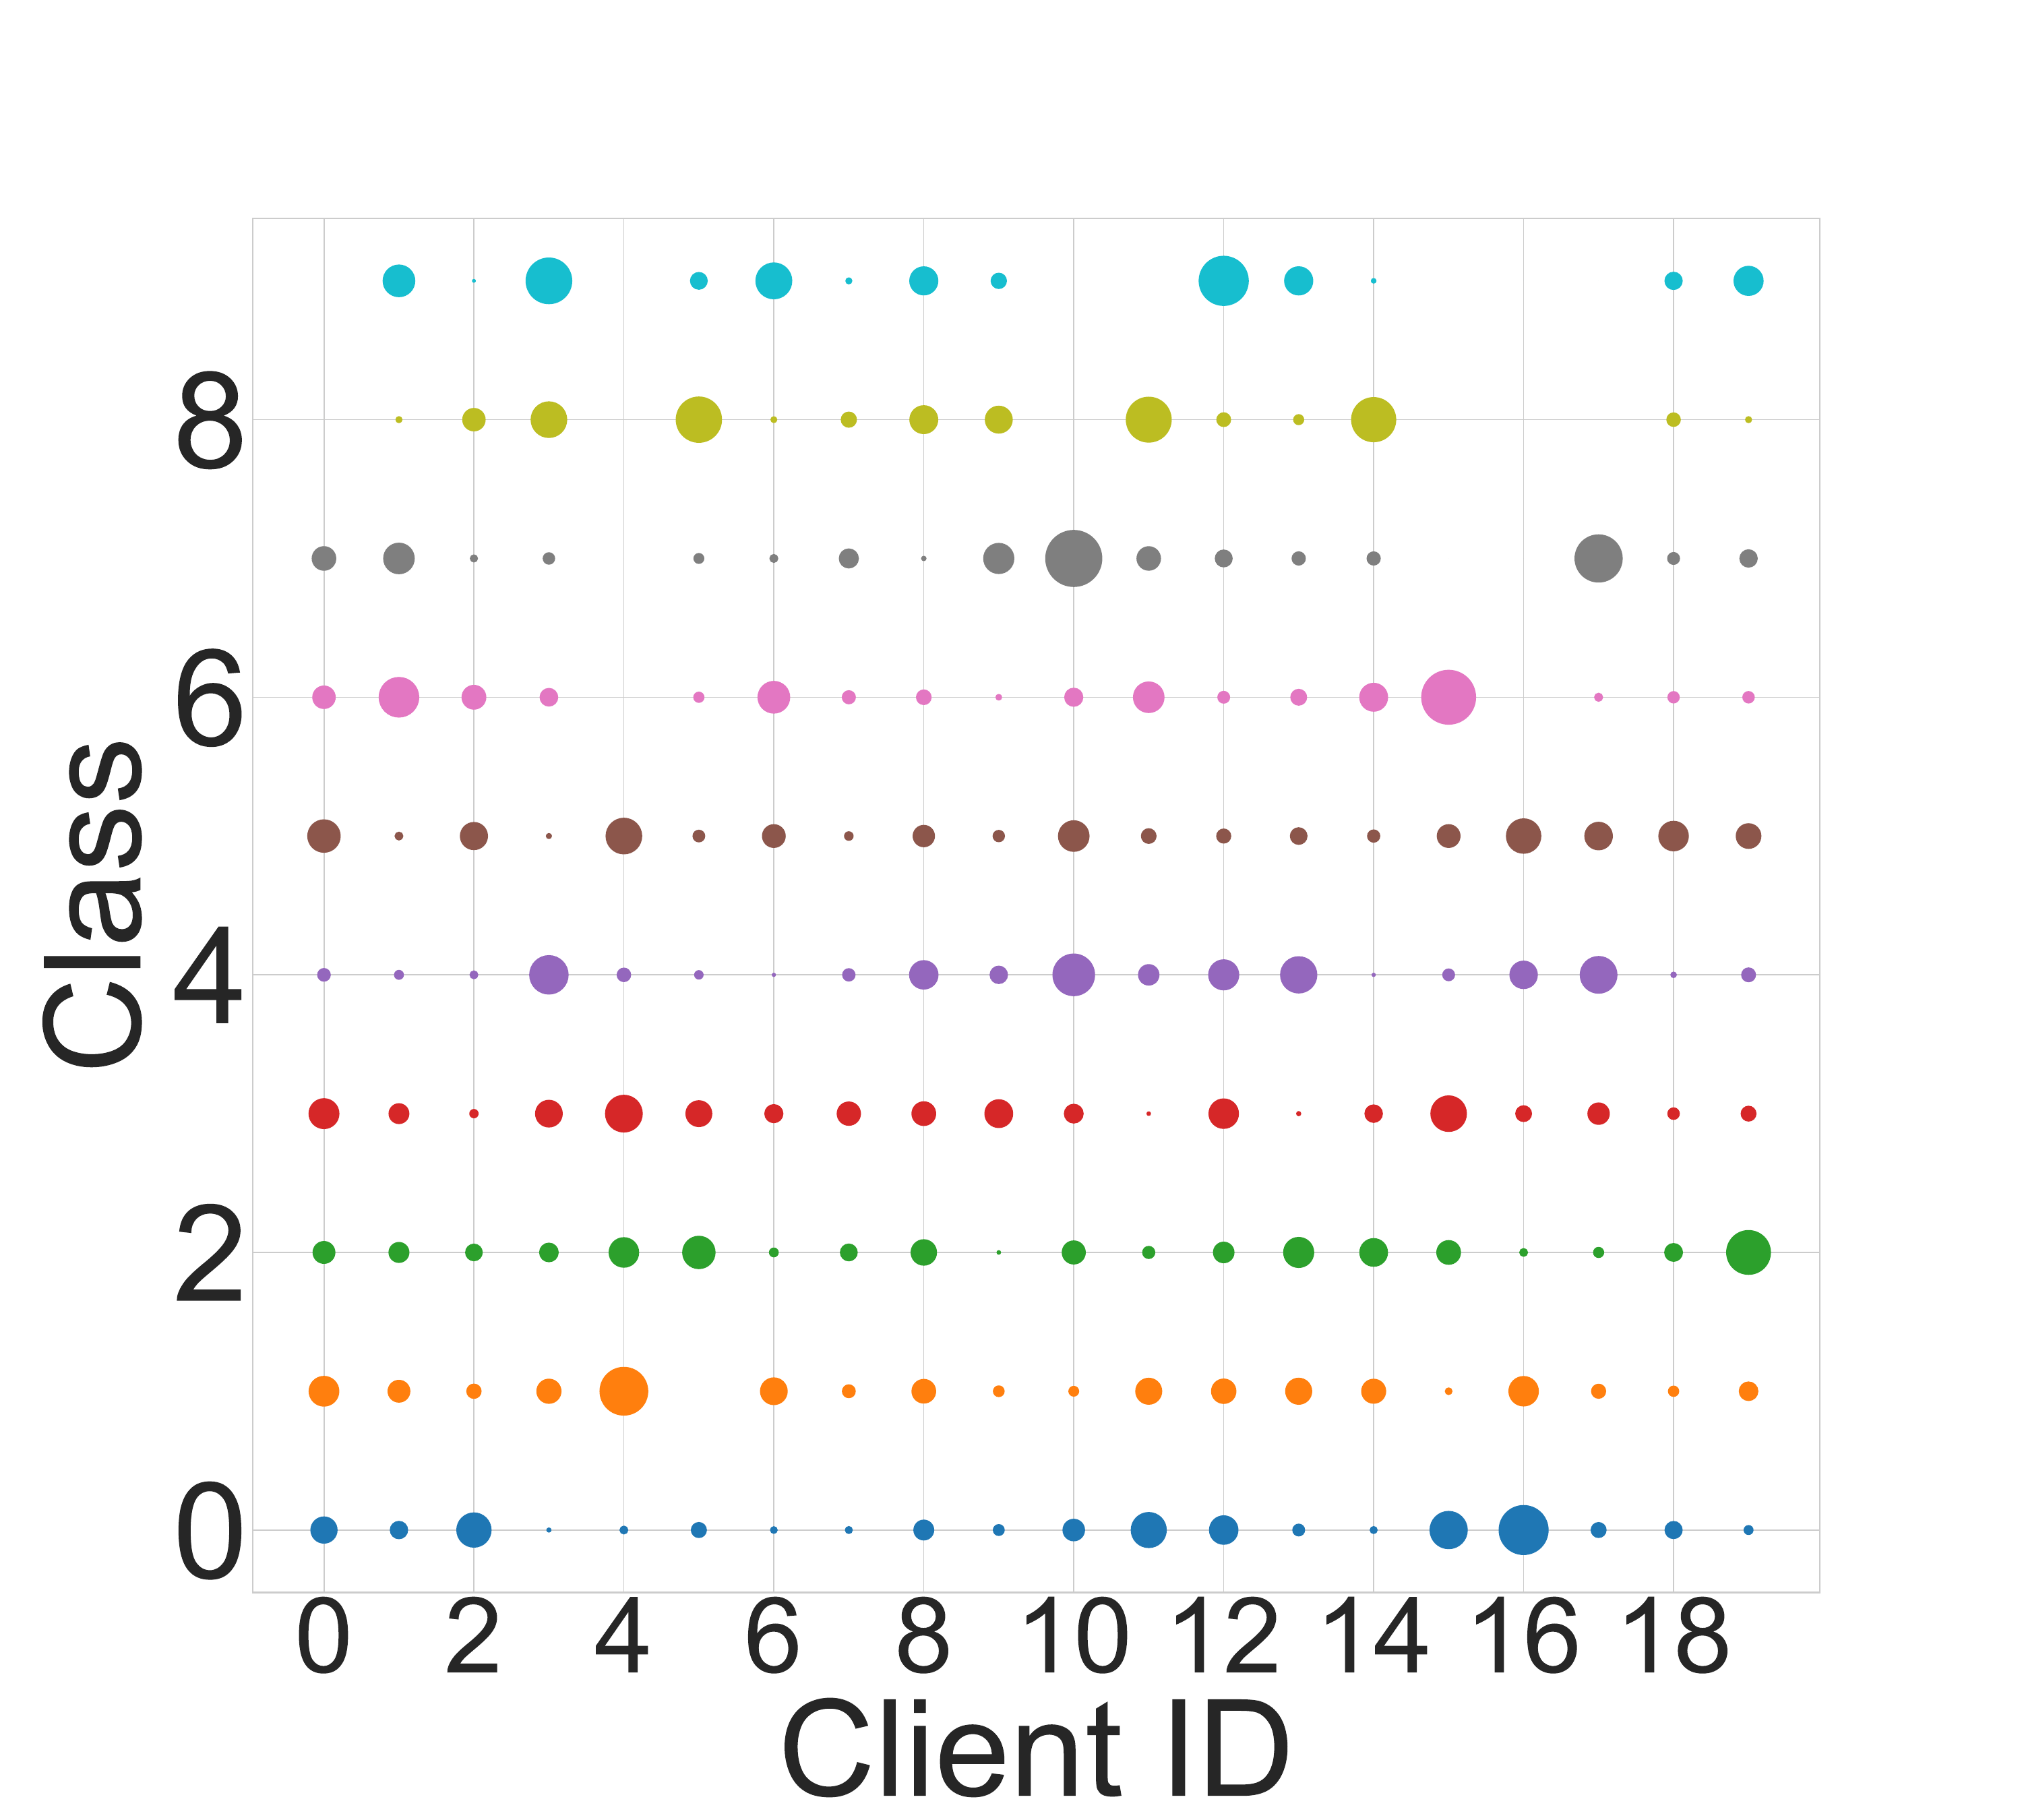}
	    \caption{
		    non-iid=1.
		}
	\end{subfigure}
	\begin{subfigure}[b]{0.3\textwidth}
        \includegraphics[width=1\textwidth]{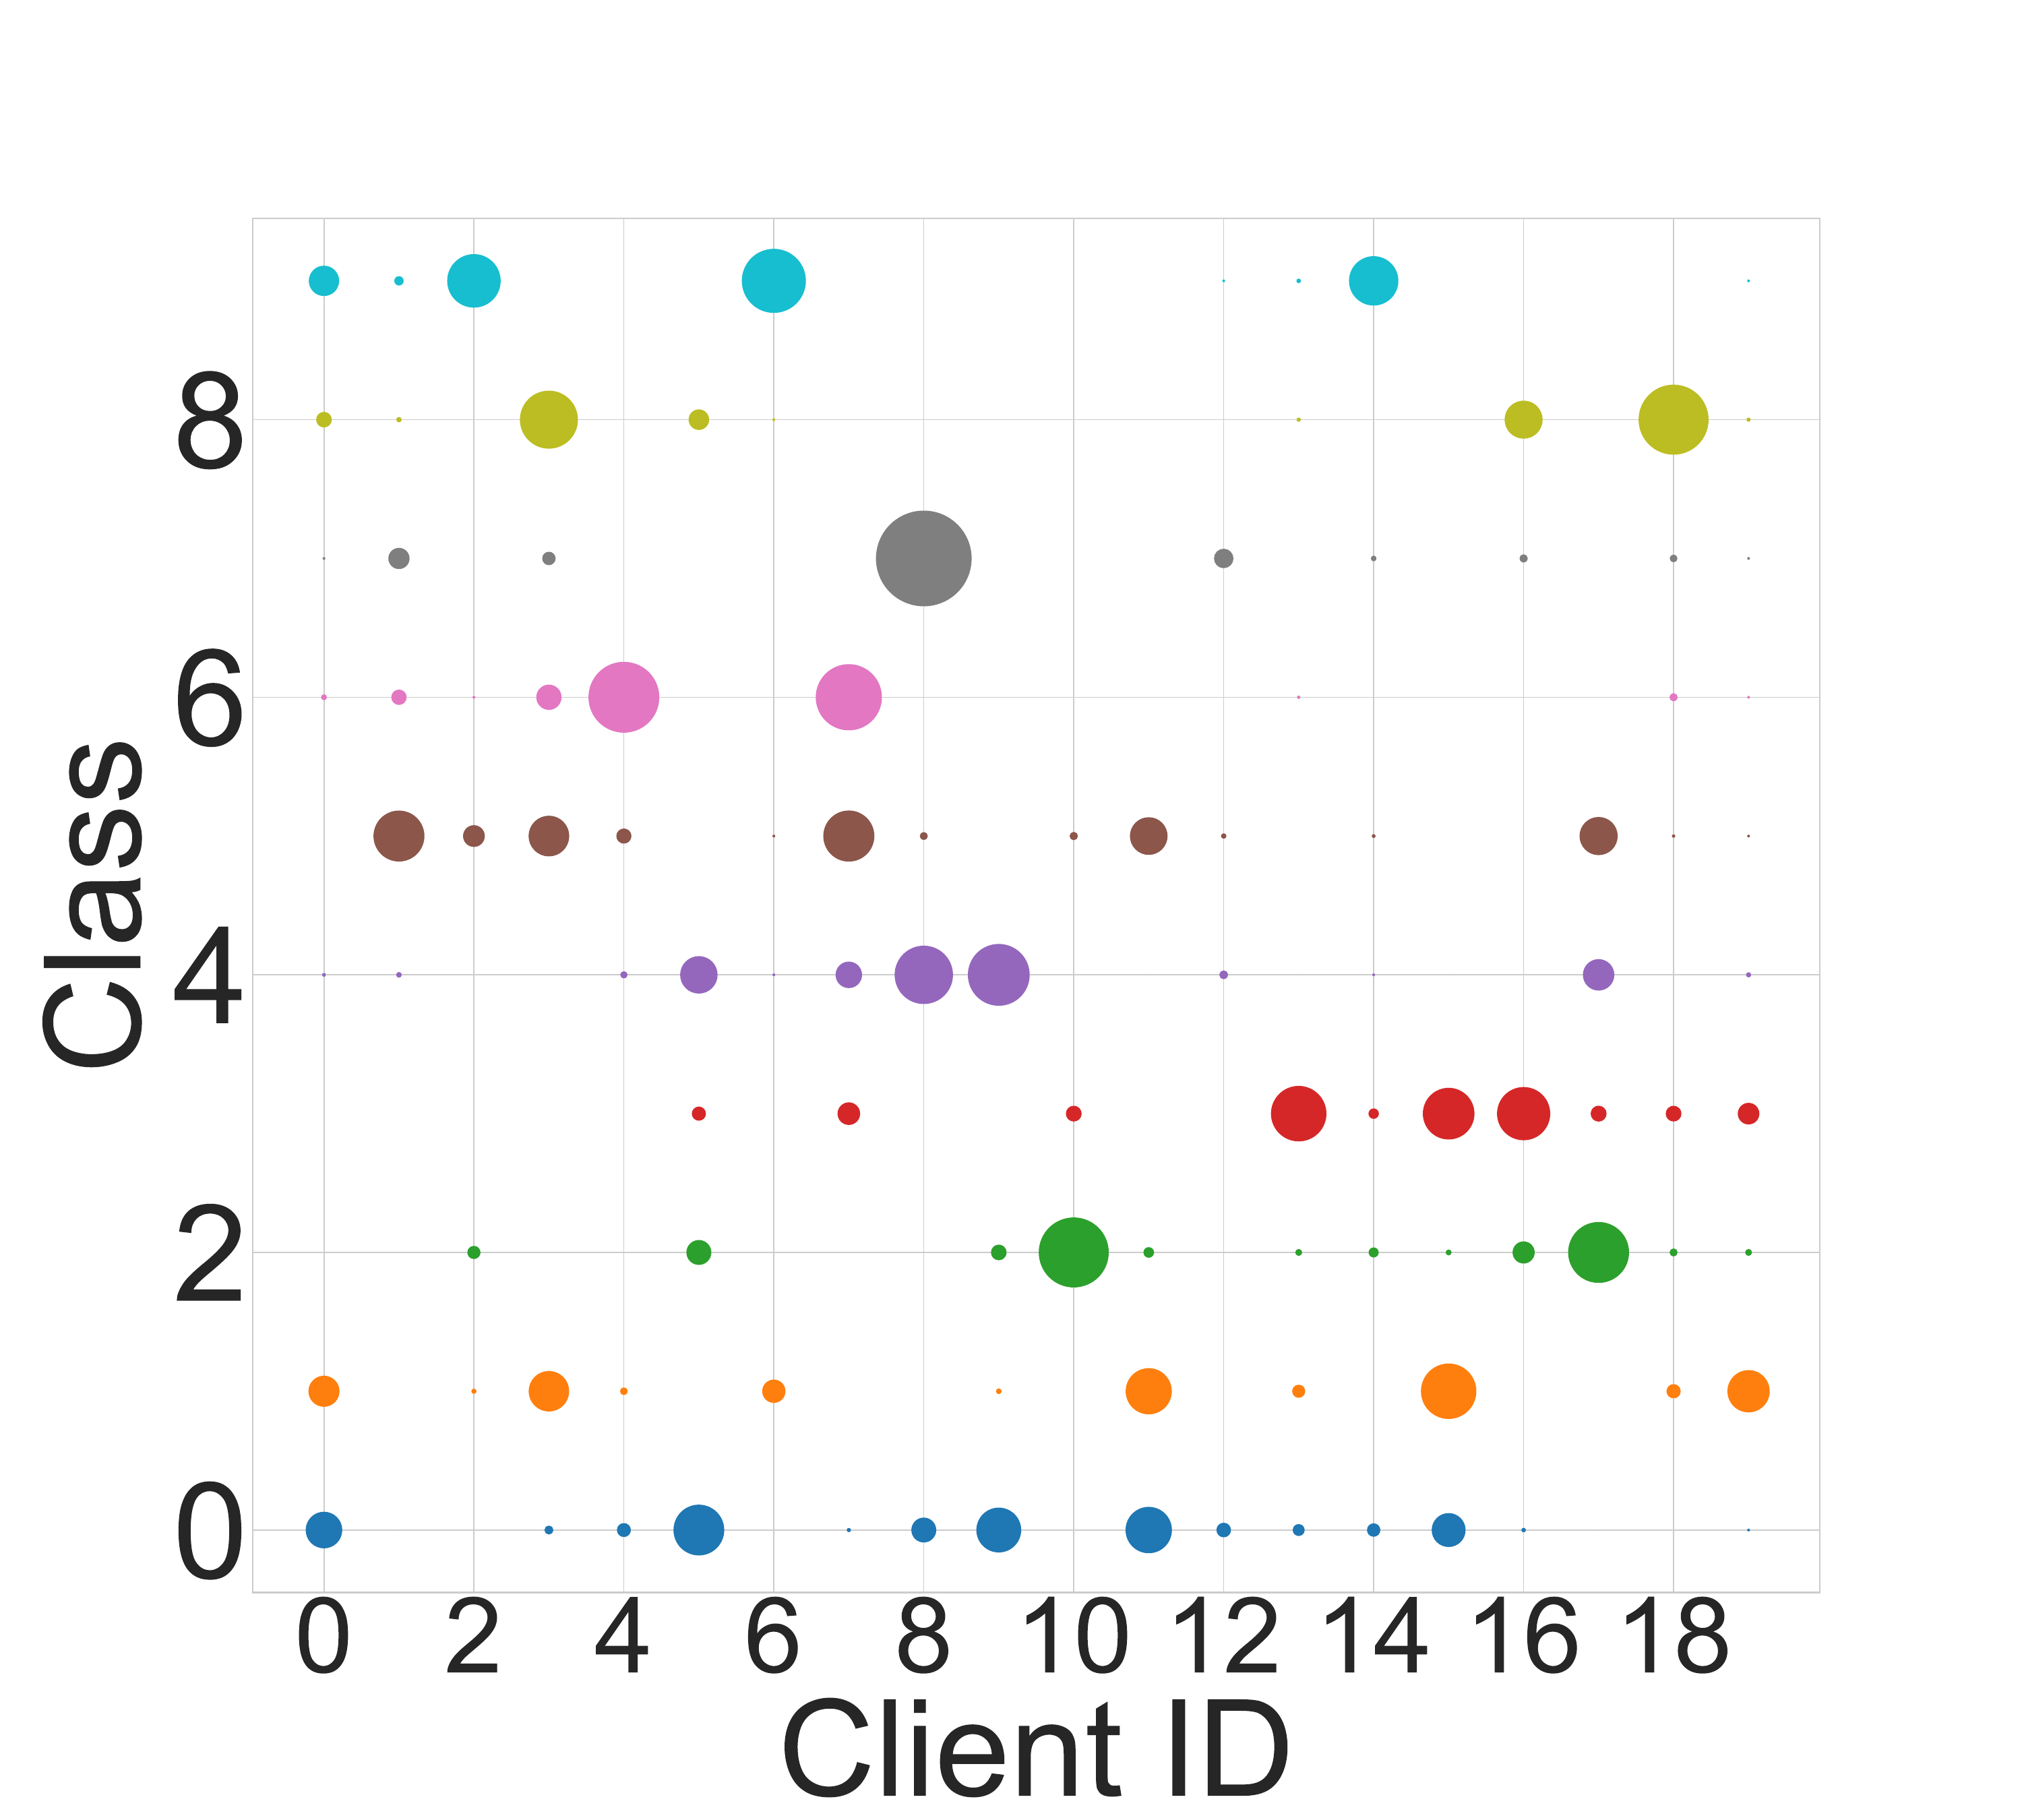}
	    \caption{
		    non-iid=0.1.
		}
	\end{subfigure}
   
    \caption{
	   \small \textbf{Non-i.i.d Degree}. Client class distribution visualization across different non-iid$=\{100, 1, 0.1\}$ values. Showing visualizations for CIFAR10 dataset partitioned using Drichlet distribution among 20 clients.
	}
	 \label{fig:client_class_distribution}
\end{figure*}
\figref{fig:client_class_distribution} visualizes the distribution of classes among 20 clients. The size of the dots symbolizes the amount of data points for that particular class in the client's dataset partition. Partition is done using Dirichlet distribution, which is parameterized by $\alpha$. 
% As seen in the figure, the lower the $\alpha$ value the higher the degree of -ness. 
Specifically for non-iid=0.1, many clients don't have even a single data point for some classes.
